# Supplementary material for: Show, Edit and Tell: A Framework for Editing Image Captions
Source: arXiv:2003.03107 source file (2020-03-06)
Supplement: Supplementary file 1 [file supp.tex]

% \documentclass[10pt,letterpaper]{article}
% \usepackage{cvpr}
% \usepackage{times}
% \usepackage{epsfig}
% \usepackage{graphicx}
% \usepackage{amsmath}
% \usepackage{amssymb}

% % Include other packages here, before hyperref.

% % If you comment hyperref and then uncomment it, you should delete
% % egpaper.aux before re-running latex.  (Or just hit 'q' on the first latex
% % run, let it finish, and you should be clear).
% \usepackage[pagebackref=true,breaklinks=true,letterpaper=true,colorlinks,bookmarks=false]{hyperref}

% \cvprfinalcopy % *** Uncomment this line for the final submission

% \def\cvprPaperID{9483} % *** Enter the CVPR Paper ID here
% \def\httilde{\mbox{\tt\raisebox{-.5ex}{\symbol{126}}}}

% % Pages are numbered in submission mode, and unnumbered in camera-ready
% \ifcvprfinal\pagestyle{empty}\fi
% \begin{document}

% %%%%%%%%% TITLE
% \title{Supplementary Material for \protect\\\textit{Show, Edit and Tell}: A Framework for Editing Image Captions}

% \maketitle


% \begin{figure*}
%     \centering
%     \includegraphics[width=0.9\textwidth,height=0.9\textheight,keepaspectratio]{suppimage}
%     \caption{Visualization of the selected words from SCMA}
%     \label{vis}
% \end{figure*}


% \section{DCNet}

% An overview of our DCNet is shown in Figure \ref{dae}. We consider the existing caption as a "noisy" caption, and wish to encode it into a compressed representation and decode the compressed representation to the desired output. Notably, an LSTM-based de-noising auto-encoder is equivalent to a Sequence-to-Sequence model. 

% For the encoder, we encode the noisy existing caption using a bi-directional LSTM and set the dimension of each direction to 512. Specifically, an existing sequence of $N$ words is first converted into a sequence of word vectors using an embedding layer: $\left[w_{1}^{S}, w_{2}^{S}, \ldots . . w_{N}^{S}\right]$ where $w_{t}^{S} \in \mathcal{R}^{1024}$, and serve as input to a bi-directional LSTM: 
% \begin{equation}
% \overrightarrow{e_{t}}=B i-L S T M\left(\overrightarrow{e_{t-1}}, w_{t}\right)
% \end{equation}
% \begin{equation}
% \overleftarrow{e_{t}}=B i-L S T M\left(\overleftarrow{e_{t+1}}, w_{t}\right)
% \end{equation}

% Which results in a matrix $E=[(\overrightarrow{e_{1}} ; \overleftarrow{e_{1}}) \ldots . (\overrightarrow{e_{N}} ; \overleftarrow{e_{N}})]$, where $;$ indicates concatenation and $E \in \mathcal{R}^{1024}$. The last hidden states of the bi-directional LSTM are concatenated and fed into a single feed-forward layer with tanh activation function:
% \begin{equation}
% E_{N}=\tanh \left(W_{O} \cdot[\overrightarrow{e_{N}} ; \overleftarrow{e_{N}}]\right)
% \end{equation}

% For the decoder, we use the Top-Down decoder \cite{Anderson2017BottomUpAT} and set the dimension size to 1024. The input to the Attention-LSTM $x_{t}^{1}$ comprise of the current word embedding, the previous hidden state of the language LSTM and the last encoder hidden state, such that $x_{t}^{1}=\left[w_{t} ; E_{N} ; h_{t-1}^{2}\right]$. The output of the attention LSTM is used to compute an attention vector over the textual features $E$:
% \begin{equation}
% c_{t}^{e}=\sum_{i=1}^{N} \alpha_{t_{i}} E_{i}
% \end{equation}
% where
% \begin{equation}
% \alpha_{t}=\operatorname{softmax}\left(w_{h}^{T} \operatorname{tanh}\left(W_{g} E+W_{k} h_{t}^{1}\right)\right)
% \end{equation}

% The output of the Attention-LSTM and the context vector $c_{t}^{e}$ serve as input to the Language-LSTM, such that: $x_{t}^{2}=\left[h_{t}^{1} ; c_{t}^{e}\right]$. The output of the Language LSTM $h_{t}^{2}$ is then fed to the output layer which predicts a word from the vocabulary. 


% \begin{figure*}
%     \centering
%     \includegraphics[width=0.9\textwidth,height=0.9\textheight,keepaspectratio]{dae}
%     \caption{An overview of our DCNet sub-module, which is an LSTM-based de-noising autoencoder.}
%     \label{dae}
% \end{figure*}

% \section{SCMA Decision Visualiztion}
% In this section, we include more results to visualize the decisions from the SCMA mechanism. Figure \ref{vis} shows the alignment plot between the existing caption and the generated caption. 

% \section{Single Model Results on COCO Online Testing Server}
% We submitted our results evaluated on the official MSCOCO testing set to the online testing server. Table 1 shows the performance of our Single Model (which includes EditNet and DCNet) on the Online COCO Test Server. For fair comparison, we directly compare our method (ETN) with other state-of-art methods which also report the scores of their single model on the Online COCO Test Server (e.g. SGAE \cite{Yang2018AutoEncodingSG}). Note that the scores reported for SGAE are for the single model (and not ensemble).

% \begin{table*}[]
% \caption{Performace of our Single Model on the Online COCO Testing Server, where B-N,
% M, R, and C are short for BLEU-N, METEOR, ROUGE-L and CIDEr-D. All values are reported as percentage (\%).}
% \begin{tabular}{|c|c|l|l|l|l|l|l|l|l|l|l|l|l|l|}
% \hline
% \textbf{Model}  & \multicolumn{2}{c|}{B-1}                                      & \multicolumn{2}{c|}{B-2}                           & \multicolumn{2}{c|}{B-3}                           & \multicolumn{2}{c|}{B-4}                           & \multicolumn{2}{c|}{M}                             & \multicolumn{2}{c|}{R}                             & \multicolumn{2}{c|}{C}                             \\ \hline
% \textbf{Metric} & c5                                 & \multicolumn{1}{c|}{c40} & \multicolumn{1}{c|}{c5} & \multicolumn{1}{c|}{c40} & \multicolumn{1}{c|}{c5} & \multicolumn{1}{c|}{c40} & \multicolumn{1}{c|}{c5} & \multicolumn{1}{c|}{c40} & \multicolumn{1}{c|}{c5} & \multicolumn{1}{c|}{c40} & \multicolumn{1}{c|}{c5} & \multicolumn{1}{c|}{c40} & \multicolumn{1}{c|}{c5} & \multicolumn{1}{c|}{c40} \\ \hline
% SCST \cite{Rennie2016SelfCriticalST}            & 78.1                               & 93.7                     & 61.9                    & 86.0                     & 47.0                    & 75.9                     & 35.2                    & 64.5                     & 27.0                    & 35.5                     & 56.3                    & 70.7                     & 114.7                   & 116.0                    \\ \hline
% LSTM-A \cite{Yao2016BoostingIC}        & 78.7                               & 93.7                     & 62.7                    & 86.7                     & 47.6                    & 76.5                     & 35.6                    & 65.2                     & 27.0                    & 35.4                     & 56.4                    & 70.5                     & 116.0                   & 118.0                    \\ \hline
% StackCap \cite{Gu2017StackCaptioningCL}      & 77.8                               & 93.2                     & 61.6                    & 86.1                     & 46.8                    & 76.0                     & 34.9                    & 64.6                     & 27.0                    & 35.6                     & 56.2                    & 70.6                     & 114.8                   & 118.3                    \\ \hline
% Up-Down \cite{Anderson2017BottomUpAT}      & 80.2                               & 95.2                     & 64.1                    & 88.8                     & 49.1                    & 79.4                     & 36.9                    & 68.5                     & 27.6                    & 36.7                     & 57.1                    & 72.4                     & 117.9                   & 120.5                    \\ \hline
% CAVP \cite{Zha2019ContextAwareVP}          & 80.1                               & 94.9                     & 64.7                    & 88.8                     & 50.0                    & 79.7                     & 37.9                    & 69.0                     & 28.1                    & 37.0                     & 58.2                    & 73.1                     & 121.6                   & 123.8                    \\ \hline
% SGAE \cite{Yang2018AutoEncodingSG}          & \multicolumn{1}{l|}{\textbf{80.6}} & \textbf{95.0}            & \textbf{65.0}           & \textbf{88.9}            & 50.1                    & 79.6                     & 37.8                    & 68.7                     & 28.1                    & 37.0                     & 58.2                    & 73.1                     & 122.7                   & 125.5                    \\ \hline
% ETN (Ours)            & \multicolumn{1}{l|}{80.3}          & 94.7                     & 64.8                    & 88.8                     & \textbf{50.2}           & \textbf{79.9}            & \textbf{38.3}           & \textbf{69.5}            & \textbf{28.6}           & \textbf{37.8}            & \textbf{58.4}           & \textbf{73.5}            & \textbf{123.6}          & \textbf{125.7}           \\ \hline
% \end{tabular}
% \end{table*}

% {\small
% \bibliographystyle{ieee_fullname}
% \bibliography{etn_final}
% }
  


% \end{document}
